# Supplementary material for: Energy Balancing of Covariate Distributions
Source: arXiv:2004.13962 source file (2022-03-11)
Supplement: Supplementary file 2 [file section_appendix.tex]

% ----------------------------------
% This section contains the appendix
% ----------------------------------

\allowdisplaybreaks

\newpage

\appendix
\addcontentsline{toc}{section}{Appendices}

% \section{Additional numerical results}
