# Supplementary material for: Energy Balancing of Covariate Distributions
Source: arXiv:2004.13962 source file (2022-03-11)
Supplement: Supplementary file 4 [file supplement.tex]

\documentclass[12pt]{article}

\usepackage{xr-hyper}
\usepackage[colorlinks, linkcolor=blue, anchorcolor=blue, citecolor=blue]{hyperref}

\usepackage{amsthm}
\usepackage[margin=0.85in]{geometry}

%% include preamble (package loading, etc)
\input{../includes/preamble}

%% include any macro definitions
\input{../includes/GrandMacros.tex}

% In your preamble
% hack for using xr with overleaf
\makeatletter
\newcommand*{\addFileDependency}[1]{% argument=file name and extension
  \typeout{(#1)}
  \@addtofilelist{#1}
  \IfFileExists{#1}{}{\typeout{No file #1.}}
}
\makeatother
 
\newcommand*{\myexternaldocument}[1]{%
    \externaldocument{#1}%
    \addFileDependency{#1.tex}%
    \addFileDependency{#1.aux}%
}

%%% for referencing things from the main text
%%% WARNING::: change to \ex ternaldocument{manuscript}
%%%           if using outside of overleaf
\myexternaldocument{manuscript}

\usepackage{titling} 

\setlength{\droptitle}{-3em}  

%\pdfminorversion=4
% NOTE: To produce blinded version, replace "1" with "0" below.
\newcommand{\blind}{1}

\begin{document}

\def\spacingset#1{\renewcommand{\baselinestretch}%
{#1}\small\normalsize} \spacingset{1}

\renewcommand{\thesection}{\Alph{section}}

%\renewcommand{\baselinestretch}{1.75}

%%%%%%%%%%%%%%%%%%%%%%%%%%%%%%%%%%%%%%%%%%%%%%%%%%%%%%%%%%%%%%%%%%%%%%%%%%%%%%

\if1\blind
{
	\title{\bf Supplementary Material for ``Energy Balancing of Covariate Distributions''}
	\author{Jared D. Huling$^{1}$\thanks{huling.7@osu.edu},
		Simon Mak$^{2}$\\
		\\
		$^{1}$Department of Statistics, The Ohio State University, Columbus, Ohio \\ [8pt]
		$^{2}$Department of Statistical Science,
		Duke University, Durham, North Carolina \\ [8pt]
	}
	\maketitle
} \fi

\if0\blind
{
	\bigskip
	\bigskip
	\bigskip
	\begin{center}
		{\Large \bf Supplementary Material for ``Energy Balancing of Covariate Distributions''}
	\end{center}
	\medskip
} \fi

\spacingset{1.75} % DON'T change the spacing!

%%%%   ------------------------------------
%%%%     Input proofs
%%%%   ------------------------------------
\input{section_07_appendix/proofs.tex}

%%%%   ------------------------------------
%%%%     Input more details about simulations/toy examples
%%%%   ------------------------------------
\input{section_04_simulation/supplement_simulation_details.tex}

%%%%   ------------------------------------
%%%%     Input more data analysis / details for analyses
%%%%   ------------------------------------
\input{section_05_analysis/section_analysis_supplement.tex}

\bibliographystyle{Chicago}
\bibliography{Bibliography}

\end{document}
